# Supplementary material for: MAVIREC: ML-Aided Vectored IR-DropEstimation and Classification
Source: arXiv:2012.10597 source file (2020-12-19)
Supplement: Supplementary file 1 [file appendix.tex]

\newpage
\appendix
{\bf List of Figures}
\begin{itemize}
   \item[1.1]  High power does not necessarily mean high IR drop (word doc coefficient features and failing testcase deep dive)
   \item[1.2]  Traditional vector based IR drop estimation flow and MAVIREC flow (demo PPT) 
   \item[2.1] Feature generation space and time decomposition (poster)
   \item[2.2] UNet 3D to 2D architecture and regression model (redraw)
   \item[4.1] ROC against PowerNet, UNet with Max, vanilla UNet 
   \item[4.2]  ROC with and without cell-based features
   \item[4.3]  ROC with and without decap features
   \item[4.4]  IR drop heatmap of MAVIREC and Redhawk (small cut portions) (weekly update slides)
   \item[4.5]  Vector profiling results on an example design list of top candidates per regions and corresponding WIR (week13 slide4)
   \item[4.6] MAVIREC (112 slices explored) coverage versus Redhawk (3 slices explored) coverage based on average power heuristic and its corresponding slice (week13 slide 11)
\end{itemize}

{\bf List of Tables}
\begin{itemize}
  \item [1.1] Runtime tables for profiling entire FSDBs comparison between commercial, PowerNet, and MAVIREC
  \item [2.1] Table listing all features used into two categories (i)~cell based and (ii)~region based features
  \item [4.1] Table summarizing designs and testbenches
  \item [4.2] Inference runtimes of PowerNet, UNet with Max, vanilla UNet, and MAVIREC
  \item [4.3] Table summarizing results for transferability on 4 different designs and test combinations based on  per instance RMSE, confusion matrix, F1 scores on 4 different testcases which are orthogonal from training set. 
  \item [4.4] Number of missed regions reported by MAVERIC. Number of false positive missed regions. Number false negative missed regions for all designs and one test each. 
\end{itemize}

{\bf List of Algorithms}
\begin{itemize}
    \item[3.1] Vector profiling flow using MAVIREC
\end{itemize}

{\bf Old results outline}
\subsection{MAVIREC versus PowerNet and baseline ML implementations}
{\it // Comparisons to include ROC, hotspot maps, for three different designs (each unseen during training cross validation), and inference runtimes between models}
\begin{itemize}
    \item PowerNet: CNN with max and average toggle rate as input, no cell-based features, regions size 1um X 1um, with decaps, and window size of 31um X 31um compared against MAVIREC with 1um X 1um size regions size with cell-based features, with decaps (no window size selection for MAVIREC).
    \item {Comparison against UNet with max structure}
    \item {Comparison against UNet}
    \item {Comparison without cell-based features}
\end{itemize}

\subsection{Impact of decaps}
\begin{itemize}
\item {Results from the model with and without decap cells as a feature}
\end{itemize}

\subsection{Vector profiling results using MAVIREC model}
\begin{itemize}
\item {Comparisons against Redhawk profiling flow due to average power and limited number of cycles explored it results missed IR drop regions. MAVIREC covers additional regions.}

\end{itemize}
